# Supplementary material for: Non-Mergeable Sketching for Cardinality Estimation
Source: arXiv:2008.08739 source file (2021-02-15)
Supplement: Supplementary file 1 [file appendix.tex]

\appendix

\section{Proof of Theorem~\ref{thm:kappa}}\label{sect:kappa}

\begin{proof}[Theorem~\ref{thm:kappa}]
First note that, by the assumptions, we have that
\begin{align*}
    \lim_{m\to\infty} \E\paren{\frac{1}{P_{m,\lambda m}}} &=  \E\paren{\lim_{m\to\infty}\frac{1}{P_{m,\lambda m}}} = \E\paren{\frac{\lambda}{\kappa_\lambda}}= \frac{\lambda}{\kappa_\lambda}.
\end{align*}
% and by a.s. convergence we also do not need this 
Also note that since $P_{m,k}$ are non-increasing as $k$ increases, by simple coupling argument, we see that for any $k\leq k'$, $\mathbb{E}\paren{1/P_{m,k}}\leq \mathbb{E}\paren{1/P_{m,k'}}$ and $\frac{\kappa_k}{k}\geq \frac{\kappa_{k'}}{k'}$.

Fix $\lambda>0$, we have, by Theorem \ref{thm:me},
\begin{align}
    \lim_{m\to\infty}\frac{1}{\lambda^2m}\Var(E_{m,\lambda m})&= \lim_{m\to\infty} \left(\frac{1}{\lambda^2m} \sum_{k=1}^{\lambda m}\E\paren{ \frac{1}{P_{m,k}}}-\frac{1}{\lambda}\right)\nonumber\\
    &=  \lim_{m\to\infty} \frac{1}{\lambda^2m} \sum_{i=0}^{\lambda-1} \sum_{j=1}^{m}
    \E\paren{\frac{1}{P_{m,im+j}}} -\frac{1}{\lambda} \label{eq:mve}
\end{align}
Since for any $j\in[1,m]$, $ \E\paren{\frac{1}{P_{m,im+j}}} \leq \E\paren{\frac{1}{P_{m,(i+1)m}}}$, we have
\begin{align*}
    \lim_{m\to\infty}\frac{1}{\lambda^2m}\Var(E_{m,\lambda m})\leq &  \lim_{m\to\infty} \frac{1}{\lambda^2m} \sum_{i=0}^{\lambda-1}  \sum_{j=1}^{m}\E\paren{\frac{1}{P_{m,(i+1)m}}} -\frac{1}{\lambda}\\
    &=    \frac{1}{\lambda^2} \sum_{i=0}^{\lambda-1}  \lim_{m\to\infty} \E\paren{\frac{1}{P_{m,(i+1)m}}} -\frac{1}{\lambda}\\
    &=    \frac{1}{\lambda^2} \sum_{i=0}^{\lambda-1}   \frac{i+1}{\kappa_{i+1}} -\frac{1}{\lambda},
\end{align*}

Denote the ARV factor as $v$.
Fix $W>0$.  Note that for any $i\in[0,\lambda/W-1]$, $\frac{k\lambda/W+i+1}{\kappa_{k\lambda/W+i+1}}\leq \frac{(k+1)\lambda/W}{\kappa_{(k+1)\lambda/W}}$. 
\begin{align}
   v \leq & \lim_{\lambda\to\infty}\left(\frac{1}{\lambda^2} \sum_{i=0}^{\lambda-1}  \frac{i+1}{\kappa_{i+1}} -\frac{1}{\lambda}\right)
    =\lim_{\lambda\to\infty}\left(\frac{1}{\lambda^2} \sum_{k=0}^{W-1}\sum_{i=0}^{\lambda/W-1}   \frac{k\lambda/W+i+1}{\kappa_{k\lambda/W+i+1}} \right)\nonumber\\
    \leq&\lim_{\lambda\to\infty}\left(\frac{1}{\lambda^2} \sum_{k=0}^{W-1}\sum_{i=0}^{\lambda/W-1}   \frac{(k+1)\lambda/W}{\kappa_{(k+1)\lambda/W}}\right)
    =\frac{1}{W^2} \sum_{k=0}^{W-1}  \lim_{\lambda\to\infty}\frac{k+1}{\kappa_{(k+1)\lambda/W}} \nonumber\\
    \intertext{note that $\lim_{\lambda\to\infty}\kappa_{(k+1)\lambda/W}=\kappa$ by the definition of scale-invariance,}
    &=\frac{1}{W^2} \sum_{k=0}^{W-1} \frac{k+1}{\kappa}= \frac{1}{2\kappa} \frac{W(W+1)}{W^2}. \label{eq:v_upper}
\end{align}

On the other hand, we can  bound it from below similarly. We will only outline the key steps since it is almost identical to the previous one. Note that for any $j\in[1,m]$, $ \E\paren{\frac{1}{P_{m,im+j}}} \geq \E\paren{\frac{1}{P_{m,im}}}$. Using this inequality in (\ref{eq:mve}), we have
\begin{align*}
    \lim_{m\to\infty}\frac{1}{\lambda^2m}\Var(E_{m,\lambda m})\geq &  \lim_{m\to\infty} \frac{1}{\lambda^2m} \sum_{i=0}^{\lambda-1}  \sum_{j=1}^{m}\E\paren{\frac{1}{P_{m,im}}} -\frac{1}{\lambda}=    \frac{1}{\lambda^2} \sum_{i=0}^{\lambda-1}   \frac{i}{\kappa_i} -\frac{1}{\lambda}.
\end{align*}
Similarly, we have
\begin{align}
    v\geq &\lim_{\lambda\to\infty}\left(\frac{1}{\lambda^2} \sum_{k=0}^{W-1}\sum_{i=0}^{\lambda/(W)-1}   \frac{k\lambda/W+i}{\kappa_{k\lambda/W+i}} \right)
    \geq\lim_{\lambda\to\infty}\left(\frac{1}{\lambda^2} \sum_{k=0}^{W-1}\sum_{i=0}^{\lambda/W-1}  \frac{k\lambda/W}{\kappa_{k\lambda/W}} \right) \nonumber\\
    &=\frac{1}{W^2} \sum_{k=0}^{W-1} \frac{k}{\kappa}= \frac{1}{2\kappa} \frac{W(W-1)}{W^2}. \label{eq:v_lower}
\end{align}

Thus by combining (\ref{eq:v_upper}) and (\ref{eq:v_lower}), we have
\begin{align*}
   \frac{1}{2\kappa} \frac{W(W-1)}{W^2}\leq v \leq \frac{1}{2\kappa} \frac{W(W+1)}{W^2}.
\end{align*}
Since the choice of $W$ is arbitrary, we conclude that the ARV factor $v$ is well-defined and  $v=\frac{1}{2\kappa}$.
\end{proof}

\ignore{
\section{Analysis of \sCurtain}\label{sect:sCurtain}
\subsection{Constant $\kappa$}
\begin{theorem}\label{thm:scurtain_kappa}
$\sCurtain$ is scale-invariant with 
\begin{align*}
    \kappa_\sCurtain=\int_{-\infty}^\infty e^{-\frac{1}{q^{t}}\frac{q^{a-1/2}+1}{q^{a-1/2}-1}} \left(1+ \varphi\paren{\frac{1}{q^{t+1}}}\right)\prod_{j=1}^\infty\left(1+\varphi\left(\frac{1}{q^{t+j(a-1/2)}}\right)\right)^2 \frac{1}{q^{t}}\frac{q-1}{q} dt,
\end{align*}
where  $\varphi(x)=\sum_{i=0}^\infty \left(e^{\frac{x}{q^{i}}\frac{q-1}{q}}-1\right)$.
\end{theorem}
\begin{proof}
Fix a cell $t$.
Let $W_2(k)$ be the height of the \emph{second} highest cell containing a dart in the $k$th column relative to column of cell $t$. 
Let $\iota = \Indicator{k \mbox{ is odd}}/2$.
We have for any $i\in\mathbb{Z}$,
\begin{align*}
    &\Pr(W_2(k)\leq t+i+\iota)\\
    &=\prod_{j\geq 1}\Pr(Y_{t+i+\iota+j,\lambda}=0) + \sum_{j\geq 1} \Pr(Y_{t+i+\iota+j,\lambda}=1)\prod_{w\geq 1,w\neq j}\Pr(Y_{t+i+\iota+w,\lambda}=0)\\
    &= \left(\prod_{j\geq 1}\Pr(Y_{t+i+\iota+j,\lambda}=0)\right)\left(1+\sum_{j\geq 1} \frac{\Pr(Y_{t+i+\iota+j,\lambda}=1)}{\Pr(Y_{t+i+\iota+j,\lambda}=0)} \right)\\
    &=e^{-\frac{\lambda}{q^{t+i+\iota+1}}} \left(1+\sum_{j\geq 1} \frac{1-e^{-\frac{\lambda}{q^{t+i+\iota+j}}\frac{q-1}{q}}}{e^{-\frac{\lambda}{q^{t+i+\iota+j}}\frac{q-1}{q}}}\right)\\
    &=e^{-\frac{\lambda}{q^{t+i+\iota+j+1}}} \left(1+\sum_{j\geq 1} \left(e^{\frac{\lambda}{q^{t+i+\iota+j}}\frac{q-1}{q}}-1\right)\right)\\
    &=e^{-\frac{\lambda}{q^{t+i+\iota+j+1}}} \left(1+\varphi\left(\frac{\lambda}{q^{t+i+\iota+j+1}}\right)\right).
\end{align*}
Now we can express the cumulative expression for the tension point $T_2$ of $\sCurtain$:
\begin{align}
    \Pr(T_2\leq i+t) &= \Pr\left(\max_{j\in\mathbb{Z}\setminus\{0\}}\{W_2(j)-|j|(a-1/2)\}\leq i+t\right) \nonumber\\
    &=\prod_{j\in\mathbb{Z}\setminus\{0\}}\Pr(W_2(j) - |j|(a-1/2)\leq i+t) \nonumber\\
    &=
    \left(\prod_{j=1}^\infty e^{-\frac{\lambda}{q^{t+i+1+j(a-1/2)}}} \left(1+\varphi\left(\frac{\lambda}{q^{t+i+1+j(a-1/2)}}\right)\right) \right)^2 \nonumber\\
    &=e^{-\frac{\lambda}{q^{t+i+1}}\frac{2}{q^{a-1/2}-1}}\prod_{j=1}^\infty\left(1+\varphi\left(\frac{\lambda}{q^{t+i+1+j(a-1/2)}}\right)\right)^2 \label{eq:t2it}
\end{align}

From the rules of $\sCurtain$, we know
\begin{align*}
   Z_{t,\lambda}&=\Indicator{Y_{t,\lambda=0}}\cdot \Indicator{t>T_2}\cdot \Indicator{t>W_2(0)}.
\end{align*}
Note that $T_2$ are independent from $Y_{t,\lambda}$ and $W_2$. We have 
\begin{align}
    \mathbb{E}(Z_{t,\lambda})&=\Pr(Y_{t,\lambda}=0,t>W_2(0))\cdot \Pr(t>T_2)\nonumber\\
    &=\left(\Pr(t>W_1(0))+\Pr(W_1(0)>t>W_2(0))\right)\cdot \Pr(T_2\leq t-1). \label{eq:EP_SC}
\end{align}
Note that
\begin{align}
   \Pr(W_1(0)>t>W_2(0))&= \Pr(Y_{t,\lambda}=0)\cdot \sum_{j\geq 1} \Pr(Y_{t+j,\lambda}=1) \prod_{k\geq 1,k\neq j}\Pr(Y_{t+k,\lambda}=0)\nonumber\\
    &=e^{-\frac{\lambda}{q^{t}}}\varphi\paren{\frac{\lambda}{q^{t+1}}},\label{eq:w1tw2}
\end{align}
and from the proof of Theorem \ref{thm:curtain-kappa} we know
\begin{align}
    \Pr(t>W_1(0))=\Pr(W_1(0)\leq t-1)=e^{-\frac{\lambda}{t}}. \label{eq:tw1}
\end{align}
Apply the expressions (\ref{eq:t2it}), (\ref{eq:w1tw2}) and (\ref{eq:tw1}) to (\ref{eq:EP_SC}) and we have
\begin{align*}
   \mathbb{E}(Z_{t,\lambda})&=e^{-\frac{\lambda}{q^{t}}\frac{2}{q^{a-1/2}-1}}\prod_{j=1}^\infty\left(1+\varphi\left(\frac{\lambda}{q^{t+j(a-1/2)}}\right)\right)^2 \left(e^{-\frac{\lambda}{q^{t}}}+ e^{-\frac{\lambda}{q^{t}}}\varphi\paren{\frac{\lambda}{q^{t+1}}}\right)\\
    &=e^{-\frac{\lambda}{q^{t}}\frac{q^{a-1/2}+1}{q^{a-1/2}-1}} \left(1+ \varphi\paren{\frac{\lambda}{q^{t+1}}}\right)\prod_{j=1}^\infty\left(1+\varphi\left(\frac{\lambda}{q^{t+j(a-1/2)}}\right)\right)^2.
\end{align*}
Then we have, from formula (\ref{eq:kappa}),
\begin{align*}
    \kappa_\sCurtain
    &=\lim_{\lambda\to\infty} \lambda\int_{-\infty}^\infty e^{-\frac{\lambda}{q^{t}}\frac{q^{a-1/2}+1}{q^{a-1/2}-1}} \left(1+ \varphi\paren{\frac{\lambda}{q^{t+1}}}\right)\prod_{j=1}^\infty\left(1+\varphi\left(\frac{\lambda}{q^{t+j(a-1/2)}}\right)\right)^2 \frac{1}{q^{t}}\frac{q-1}{q} dt\\
    &=\int_{-\infty}^\infty e^{-\frac{1}{q^{t}}\frac{q^{a-1/2}+1}{q^{a-1/2}-1}} \left(1+ \varphi\paren{\frac{1}{q^{t+1}}}\right)\prod_{j=1}^\infty\left(1+\varphi\left(\frac{1}{q^{t+j(a-1/2)}}\right)\right)^2 \frac{1}{q^{t}}\frac{q-1}{q} dt.
\end{align*}
\end{proof}

\subsection{Average Number of  Bits Per column}
Each column uses $\log_2(2a)$ bits to store its offset in the second curtain. 
Note that $\sCurtain$ uses the unary encoding to store the distance between the highest cell and the curtain.  Next, we analyze the average number of 
bits $\sCurtain$ uses per column for the unary encoding. 

Let $r\in[0,1)$ be the offset. We call the column with cells of  height $\{i+r\mid i\in\mathbb{Z}\}$ as \emph{column $r$}. Note that $W_1(0)$, $W_2(0)$ and $T_2$ can be defined for column $r$ by using any cell in that column as the reference cell. When in tension, it takes $\max(W_1(0)-T_2+1,1)$ bits to store the distance in the $\delta$ vector. 
When not in tension, it takes $(W_1(0)-W_2(0))$ bits.  Let $K_r$ be  the number of bits for the unary coding for a column $r$. Thus we have
\begin{align*}
    K_r=\Indicator{W_2(0)\leq T_2}\max(W_1(0)-T_2+1,1)+\Indicator{W_2(0)> T_2}(W_1(0)-W_2(0)).
\end{align*}

\begin{theorem}\label{thm:scurtain_unary}
The average unary encoding length is independent from $\lambda$. Specifically,
\begin{align*}
    \int_0^1\E(K_r) dr=1+\int_{-\infty}^\infty e^{-\frac{\lambda}{q^{t}}\frac{2}{q^{a-1/2}-1}}\prod_{j=1}^\infty\left(1+\varphi\left(\frac{\lambda}{q^{t+j(a-1/2)}}\right)\right)^2 \left(e^{-\frac{\lambda}{q^{t}}}\varphi\paren{\frac{\lambda}{q^{t}}}-\left(e^{-\frac{\lambda}{q^{t+1}}}-e^{-\frac{\lambda}{q^{t}}}\right)\varphi\paren{\frac{\lambda}{q^{t+1}}}\right)dt.
\end{align*}
\end{theorem}
\begin{proof}
For simplicity, we write $W_1(0)$ and $W_2(0)$ as $W_1$ and $W_2$. We also write $T_2$ as $T$. Note that $T$ is independent from $W_1$ and $W_2$.

First we note that 
\begin{align*}
    \max(W_1-T+1,1)=1+\Indicator{W_1\geq T}(W_1-T).
\end{align*}
Then we have
\begin{align}
    K_r&=\left(\Indicator{W_1\geq T}(W_1-T)+1\right)\Indicator{W_2\leq T} + (W_1-W_2)\Indicator{W_2> T} \nonumber\\
    &=\Indicator{W_2\leq T}+\sum_{i=-\infty}^\infty \left( \Indicator{W_2\leq T} \Indicator{W_1\geq r+ i>T}  + \Indicator{W_2> T}\Indicator{W_1\geq r+ i>W_2} \right) \nonumber\\
    &=\Indicator{W_2\leq T}+\sum_{i=-\infty}^\infty \Indicator{r+i>T}\Indicator{W_1\geq r+i>W_2}. \label{eq:codef}
\end{align}

Note that we have
\begin{align}
    \Pr(W_1\geq r+ i>W_2)&=\sum_{j\geq0} \Pr(Y_{i+r+j,\lambda}=1) \prod_{k\geq 0,k\neq j}\Pr(Y_{i+r+k,\lambda}=0)
    =e^{-\frac{\lambda}{q^{i+r}}}\varphi\paren{\frac{\lambda}{q^{i+r}}},\label{eq:code1}
\end{align}
\begin{align}
    \Pr(W_2\leq T) &= \sum_{i=-\infty}^\infty \Pr(T\geq r+ i) \Pr(W_2= r+ i)= 1- \sum_{i=-\infty}^\infty \Pr(T< r+i) \Pr(W_2=r+ i),\label{eq:code2}
\end{align}
and 
\begin{align}
    \Pr(W_2= r+i)&=\Pr(Y_{r+i,\lambda}=1)\sum_{j\geq 1} \Pr(Y_{r+i+j,\lambda}=1) \prod_{k\geq 1,k\neq j}\Pr(Y_{r+i+k,\lambda}=0)\nonumber\\
    &=\left(1-e^{-\frac{\lambda}{q^{r+i}}\frac{q-1}{q}}\right)e^{-\frac{\lambda}{q^{r+i+1}}}\varphi\paren{\frac{\lambda}{q^{r+i+1}}}\nonumber\\
    &=\left(e^{-\frac{\lambda}{q^{r+i+1}}}-e^{-\frac{\lambda}{q^{r}}}\right)\varphi\paren{\frac{\lambda}{q^{r+i+1}}}.\label{eq:code3}
\end{align}
Apply the expressions (\ref{eq:code1}), (\ref{eq:code2}) and (\ref{eq:code3}) to (\ref{eq:codef}) and we have,
\begin{align*}
    &\mathbb{E}(K_r) \\
    &= \mathbb{E}\paren{\Indicator{W_2\leq T}+\sum_{i=-\infty}^\infty \Indicator{r+i>T}\Indicator{W_1\geq r+i>W_2}}\\
    &=\Pr(W_2\leq T)+\sum_{i=-\infty}^\infty \Pr(i>T)\Pr(W_1\geq i>W_2)\\
    &=1+\sum_{i=-\infty}^\infty \Pr(r+i>T)\left(\Pr(W_1\geq r+i>W_2) -\Pr(W_2= r+i)\right)\\
    &=1+\sum_{i=-\infty}^\infty e^{-\frac{\lambda}{q^{i+r}}\frac{2}{q^{a-1/2}-1}}\prod_{j=1}^\infty\left(1+\varphi\left(\frac{\lambda}{q^{i+r+j(a-1/2)}}\right)\right)^2 \left(e^{-\frac{\lambda}{q^{i+r}}}\varphi\paren{\frac{\lambda}{q^{i+r}}}-\left(e^{-\frac{\lambda}{q^{i+r+1}}}-e^{-\frac{\lambda}{q^{i+r}}}\right)\varphi\paren{\frac{\lambda}{q^{i+r+1}}}\right) .
\end{align*}
Finally, due to smoothing, we have (set $t=i+r$)
\begin{align*}
    &\int_0^1 \mathbb{E}(K_r)  dr \nonumber \\
    &= 1+\int_{-\infty}^\infty e^{-\frac{\lambda}{q^{t}}\frac{2}{q^{a-1/2}-1}}\prod_{j=1}^\infty\left(1+\varphi\left(\frac{\lambda}{q^{t+j(a-1/2)}}\right)\right)^2 \left(e^{-\frac{\lambda}{q^{t}}}\varphi\paren{\frac{\lambda}{q^{t}}}-\left(e^{-\frac{\lambda}{q^{t+1}}}-e^{-\frac{\lambda}{q^{t}}}\right)\varphi\paren{\frac{\lambda}{q^{t+1}}}\right)dt. \label{eq:ek}
\end{align*}
\end{proof}

By numerical evaluations, the optimal parametrization such that $a$ is a power of 2 is about $(q,a)=(2.2,2)$. Taking these parameters, we have $\kappa_{\sCurtain}\approx 0.937$ and the average number of bits per sketch $3.86$. Applying Theorem \ref{thm:kappa}, we get its $\MVP$ $\frac{3.86}{2\cdot 0.937}\approx 2.06$.
}
